# Supplementary material for: Structural-Spectral Graph Convolution with Evidential Edge Learning for Hyperspectral Image Clustering
Source: arXiv:2506.09920 source file (2025-11-20)
Supplement: Supplementary file 1 [file supplementary_file.tex]

\documentclass[onecolumn,journal]{IEEEtran}
\usepackage{amsmath, amsfonts}
\usepackage{orcidlink}

% hyperlink
\usepackage[nocompress]{cite}
\hypersetup{
colorlinks,
citecolor=blue,
linkcolor=blue,
urlcolor=blue
}

\usepackage{mathrsfs}
\usepackage{algorithmic}
\usepackage{amssymb}
\usepackage{algorithm}
\usepackage{array}
\usepackage[caption=false, font=normalsize, labelfont=rm, textfont=rm]{subfig}
\usepackage{textcomp}
\usepackage{stfloats}
\usepackage{url}
\usepackage{bm}
\usepackage{verbatim}
\usepackage{graphicx}
\usepackage{siunitx}
\usepackage{graphicx}
\usepackage[normalem]{ulem}
\usepackage{array}
\usepackage{makecell}
\usepackage{multirow}
\usepackage{booktabs}

\hyphenation{op-tical net-works semi-conduc-tor IEEE-Xplore}

\begin{document}

\title{Supplementary Material for Structural-Spectral Graph Convolution with Evidential Edge Learning for Hyperspectral Image Clustering}

\author{
  Jianhan~Qi$^{\orcidlink{0009-0004-3810-083X}}$,
  Yuheng~Jia$^{\orcidlink{0000-0002-3907-6550}}$,~\IEEEmembership{Member,~IEEE,}
  Hui~Liu$^{\orcidlink{0000-0003-2159-025X}}$,
  Junhui~Hou$^{\orcidlink{0000-0003-3431-2021}}$,~\IEEEmembership{Senior Member,~IEEE}
}

% \onecolumn

\maketitle

\section{Visualizations of Clustering Map}
In this section, we present the clustering map visualizations of our method and the compared methods on \textit{Pavia University}, \textit{Botswana} and \textit{Trento}. As shown in Figs. \ref{PU_clustering_map}, \ref{BO_clustering_map} and \ref{TR_clustering_map}, our method generates clustering maps that are closest to the ground truth, demonstrating its effectiveness and superiority.

\begin{figure}[h]
  \centering
  \hfill
  \subfloat[]{\includegraphics[width=0.076\textwidth]{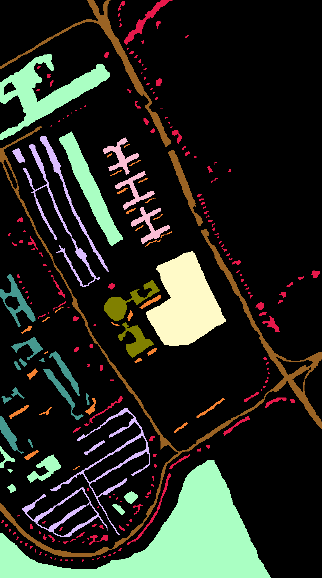}\label{PU_gt}}
  \hfill
  \subfloat[]{\includegraphics[width=0.076\textwidth]{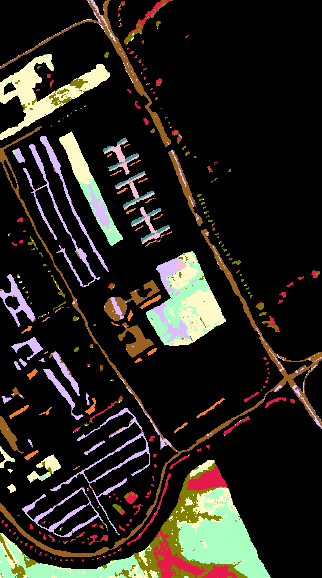}\label{PU_kmeans}}
  \hfill
  \subfloat[]{\includegraphics[width=0.076\textwidth]{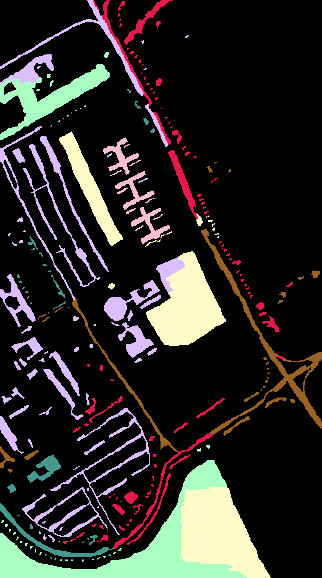}\label{PU_ssc}}
  \hfill
  \subfloat[]{\includegraphics[width=0.076\textwidth]{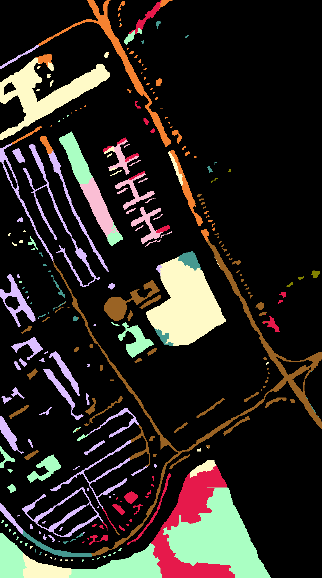}\label{PU_ncsc}}
  \hfill
  \subfloat[]{\includegraphics[width=0.076\textwidth]{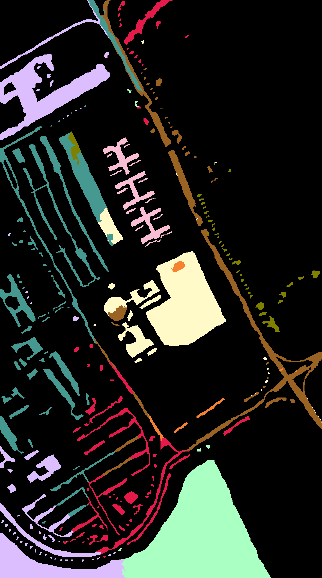}\label{PU_sglsc}}
  \hfill
  \subfloat[]{\includegraphics[width=0.076\textwidth]{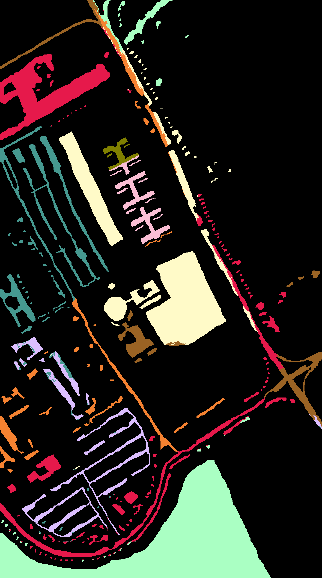}\label{PU_dgae}}
  \hfill
  \subfloat[]{\includegraphics[width=0.076\textwidth]{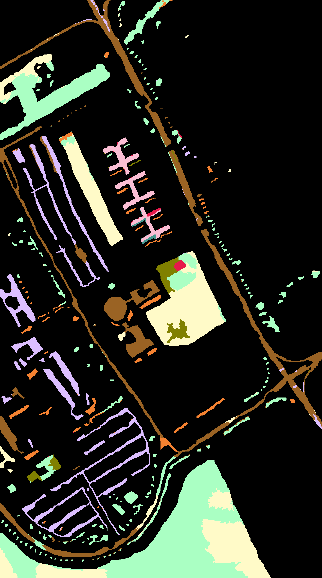}\label{PU_egrc}}
  \hfill
  \subfloat[]{\includegraphics[width=0.076\textwidth]{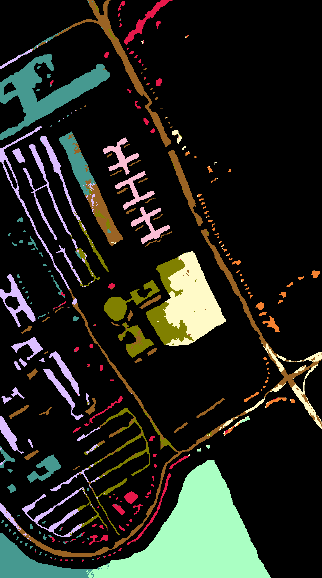}\label{PU_s3ulda}}
  \hfill
  \subfloat[]{\includegraphics[width=0.076\textwidth]{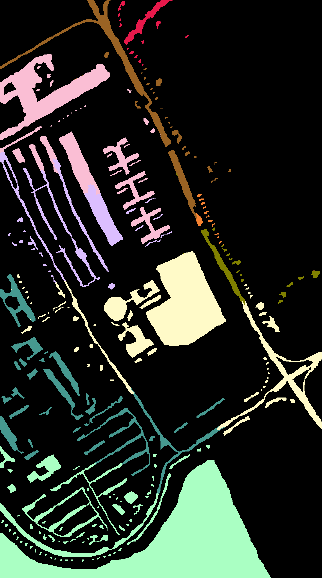}\label{PU_s2dl}}
  \hfill
  \subfloat[]{\includegraphics[width=0.076\textwidth]{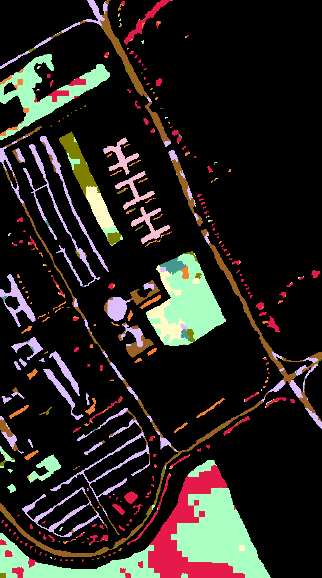}\label{PU_sdst}}
  \hfill
  \subfloat[]{\includegraphics[width=0.076\textwidth]{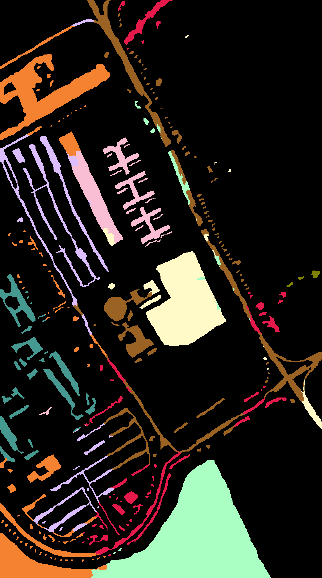}\label{PU_spgcc}}
  \hfill
  \subfloat[]{\includegraphics[width=0.076\textwidth]{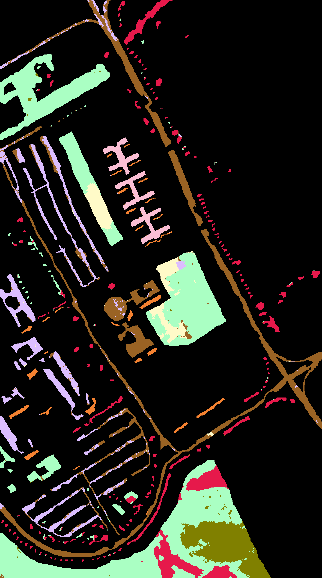}\label{PU_sapc}}
  \hfill
  \subfloat[]{\includegraphics[width=0.076\textwidth]{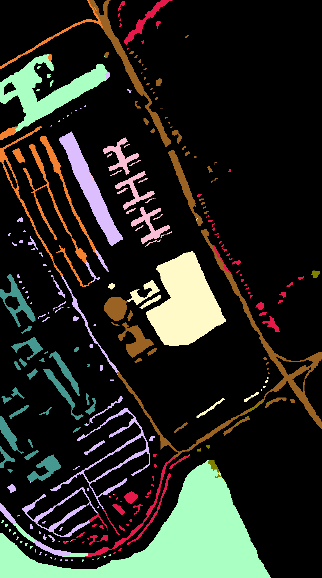}\label{PU_our}}
  \hfill
  \caption{Clustering maps on \textit{Pavia University}: (a) ground truth, (b) K-means, (c) SSC, (d) NCSC, (e) SGLSC, (f) DGAE, (g) EGRC, (h) S$^3$-ULDA, (i) S$^2$DL, (j) SDST, (k) SPGCC, (l) SAPC, (m) Ours.}
  \label{PU_clustering_map}
\end{figure}

\begin{figure}[h]
  \centering
  \hfill
  \subfloat[]{\includegraphics[width=0.076\textwidth]{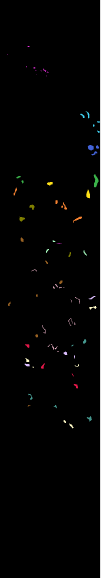}\label{BO_gt}}
  \hfill
  \subfloat[]{\includegraphics[width=0.076\textwidth]{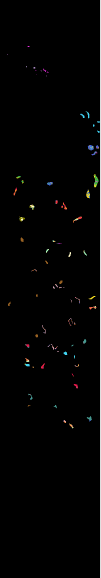}\label{BO_kmeans}}
  \hfill
  \subfloat[]{\includegraphics[width=0.076\textwidth]{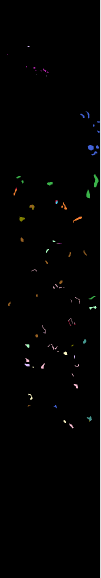}\label{BO_ssc}}
  \hfill
  \subfloat[]{\includegraphics[width=0.076\textwidth]{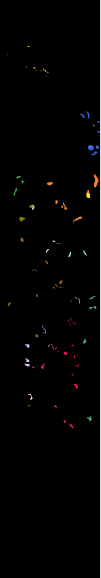}\label{BO_ncsc}}
  \hfill
  \subfloat[]{\includegraphics[width=0.076\textwidth]{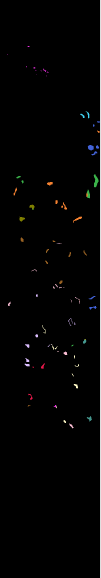}\label{BO_sglsc}}
  \hfill
  \subfloat[]{\includegraphics[width=0.076\textwidth]{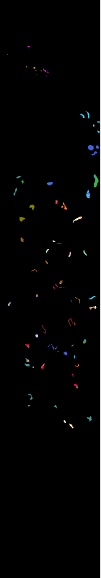}\label{BO_dgae}}
  \hfill
  \subfloat[]{\includegraphics[width=0.076\textwidth]{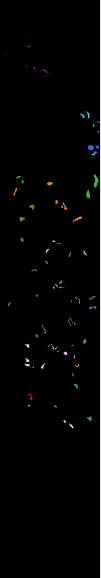}\label{BO_egrc}}
  \hfill
  \subfloat[]{\includegraphics[width=0.076\textwidth]{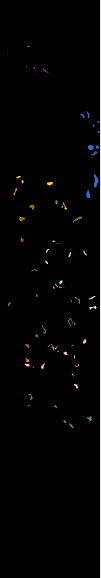}\label{BO_s3ulda}}
  \hfill
  \subfloat[]{\includegraphics[width=0.076\textwidth]{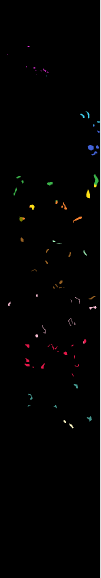}\label{BO_s2dl}}
  \hfill
  \subfloat[]{\includegraphics[width=0.076\textwidth]{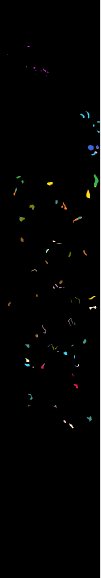}\label{BO_sdst}}
  \hfill
  \subfloat[]{\includegraphics[width=0.076\textwidth]{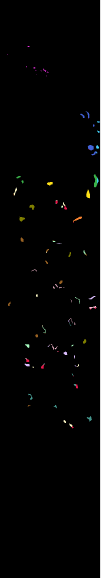}\label{BO_spgcc}}
  \hfill
  \subfloat[]{\includegraphics[width=0.076\textwidth]{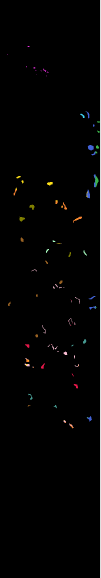}\label{BO_sapc}}
  \hfill
  \subfloat[]{\includegraphics[width=0.076\textwidth]{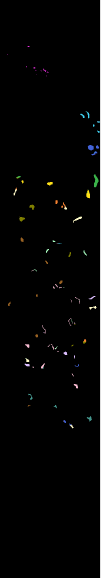}\label{BO_our}}
  \hfill
  \caption{Clustering maps on \textit{Botswana}: (a) ground truth, (b) K-means, (c) SSC, (d) NCSC, (e) SGLSC, (f) DGAE, (g) EGRC, (h) S$^3$-ULDA, (i) S$^2$DL, (j) SDST, (k) SPGCC, (l) SAPC, (m) Ours.}
  \label{BO_clustering_map}
\end{figure}

\clearpage

\begin{figure}[t]
  \centering
  \hfill
  \subfloat[]{\includegraphics[width=0.076\textwidth]{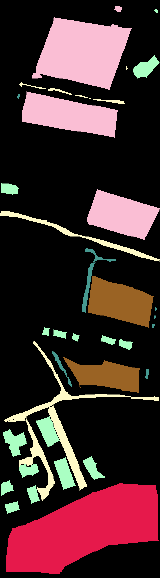}\label{TR_gt}}
  \hfill
  \subfloat[]{\includegraphics[width=0.076\textwidth]{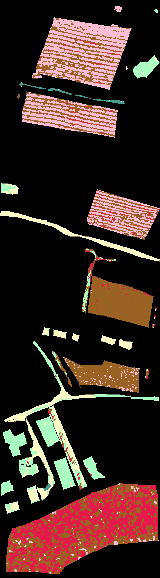}\label{TR_kmeans}}
  \hfill
  \subfloat[]{\includegraphics[width=0.076\textwidth]{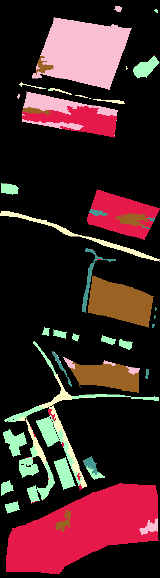}\label{TR_ssc}}
  \hfill
  \subfloat[]{\includegraphics[width=0.076\textwidth]{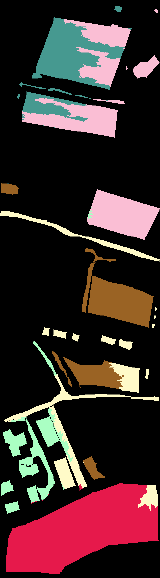}\label{TR_ncsc}}
  \hfill
  \subfloat[]{\includegraphics[width=0.076\textwidth]{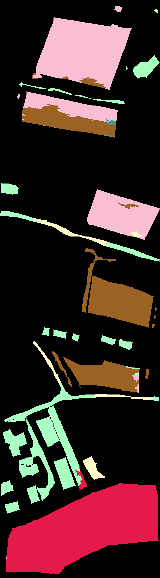}\label{TR_sglsc}}
  \hfill
  \subfloat[]{\includegraphics[width=0.076\textwidth]{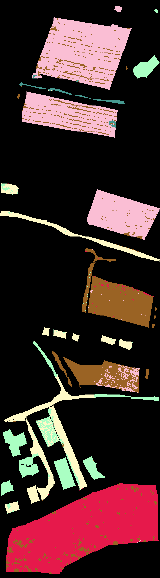}\label{TR_dgae}}
  \hfill
  \subfloat[]{\includegraphics[width=0.076\textwidth]{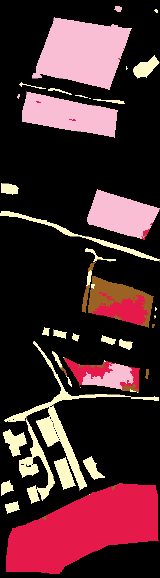}\label{TR_egrc}}
  \hfill
  \subfloat[]{\includegraphics[width=0.076\textwidth]{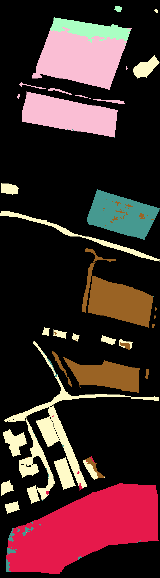}\label{TR_s3ulda}}
  \hfill
  \subfloat[]{\includegraphics[width=0.076\textwidth]{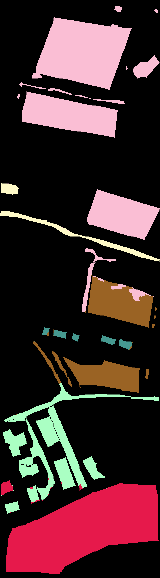}\label{TR_s2dl}}
  \hfill
  \subfloat[]{\includegraphics[width=0.076\textwidth]{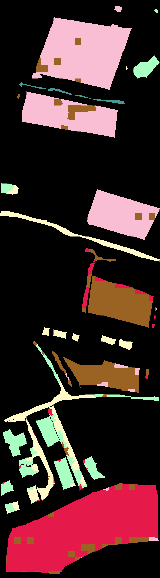}\label{TR_sdst}}
  \hfill
  \subfloat[]{\includegraphics[width=0.076\textwidth]{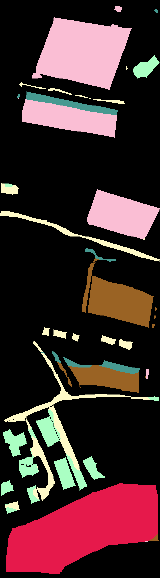}\label{TR_spgcc}}
  \hfill
  \subfloat[]{\includegraphics[width=0.076\textwidth]{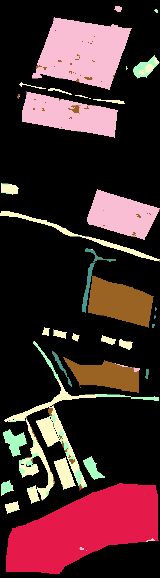}\label{TR_sapc}}
  \hfill
  \subfloat[]{\includegraphics[width=0.076\textwidth]{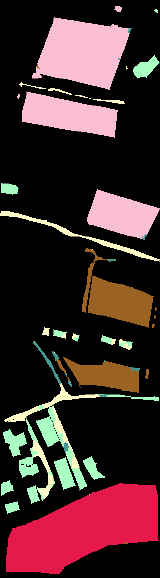}\label{TR_our}}
  \hfill
  \caption{Clustering maps on \textit{Trento}: (a) ground truth, (b) K-means, (c) SSC, (d) NCSC, (e) SGLSC, (f) DGAE, (g) EGRC, (h) S$^3$-ULDA, (i) S$^2$DL, (j) SDST, (k) SPGCC, (l) SAPC, (m) Ours.}
  \label{TR_clustering_map}
\end{figure}

\section{Visualizations of Superpixel Embeddings with t-SNE}
t-distributed stochastic neighbor embedding (t-SNE) \cite{tsne} is used for the visualization of superpixel embeddings. We report the visualization results of raw features and our method learned embeddings. As shown in Fig. \ref{tsne}, visualizations of raw features exhibit highly overlapped clusters, confirming the severe spectral confusion in the initial data. This directly corresponds to their low clustering accuracy. In contrast, our learned embeddings demonstrate a far more structured and meaningful feature space. Regarding intra-cluster compactness, superpixels belonging to the same class are grouped into tight and dense clusters. As for inter-cluster separability, the distance between different clusters is significantly enlarged, resulting in clear margins. This comparison provides strong evidence that our method can learn superior discriminative representations for clustering.

\begin{figure}[h]
  \centering
  \subfloat[]{\includegraphics[width=0.24\textwidth]{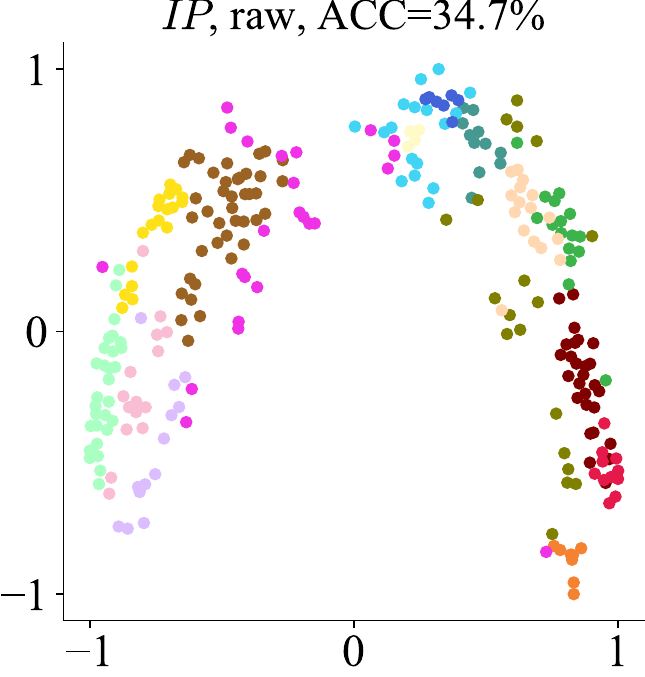}}
  \hfill
  \subfloat[]{\includegraphics[width=0.24\textwidth]{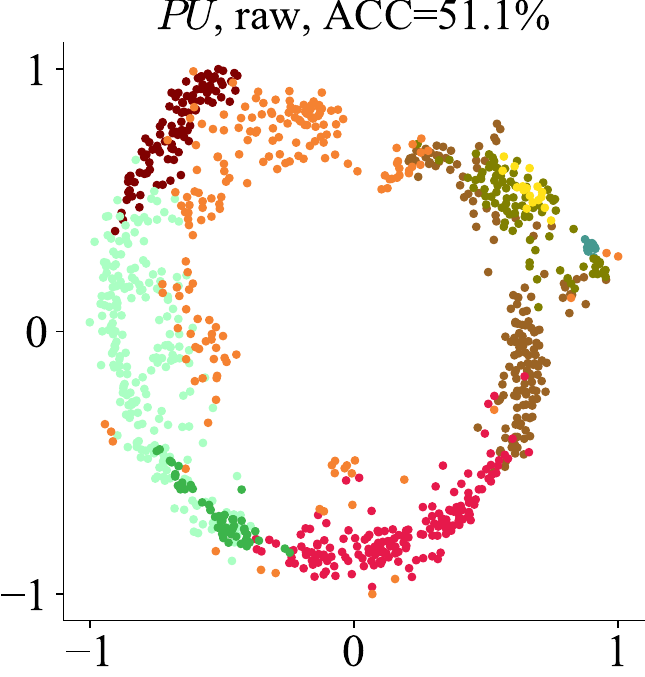}}
  \hfill
  \subfloat[]{\includegraphics[width=0.24\textwidth]{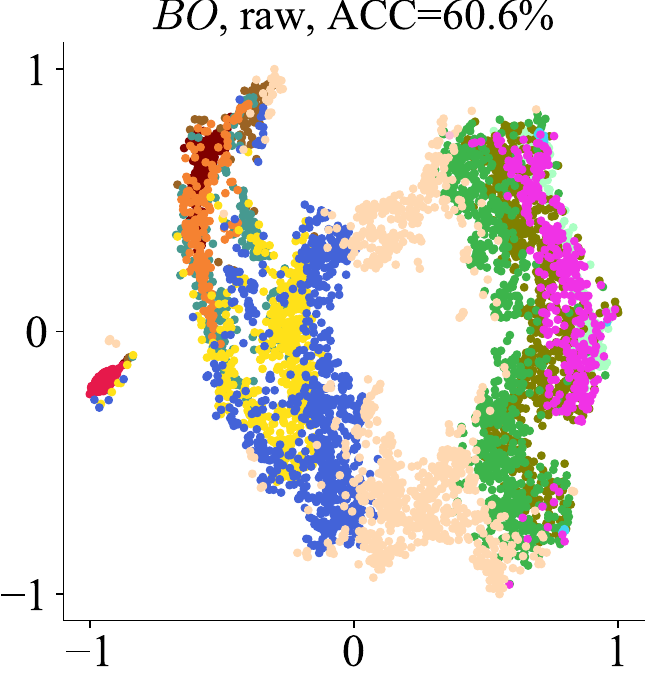}}
  \hfill
  \subfloat[]{\includegraphics[width=0.24\textwidth]{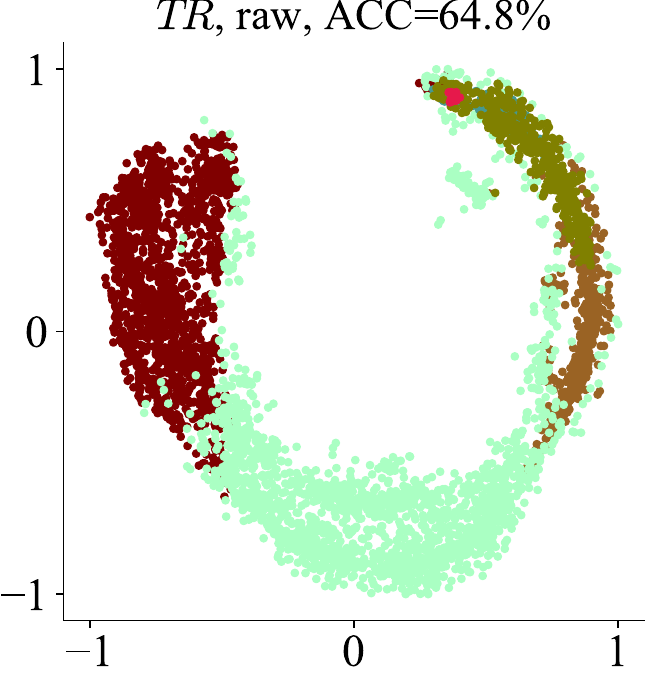}}
  \\
  \subfloat[]{\includegraphics[width=0.24\textwidth]{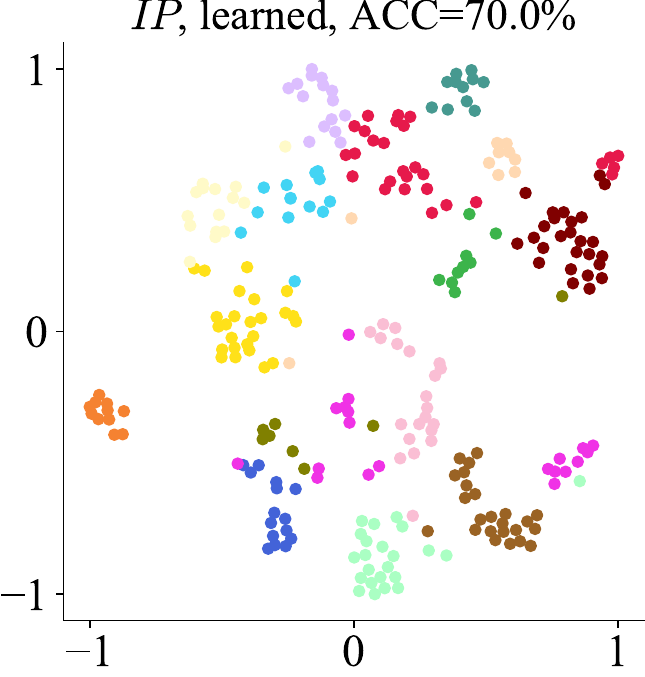}}
  \hfill
  \subfloat[]{\includegraphics[width=0.24\textwidth]{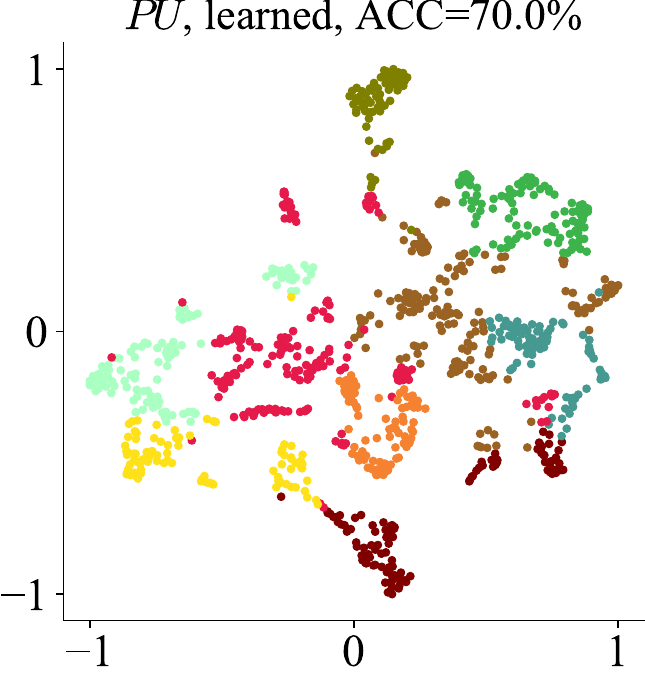}}
  \hfill
  \subfloat[]{\includegraphics[width=0.24\textwidth]{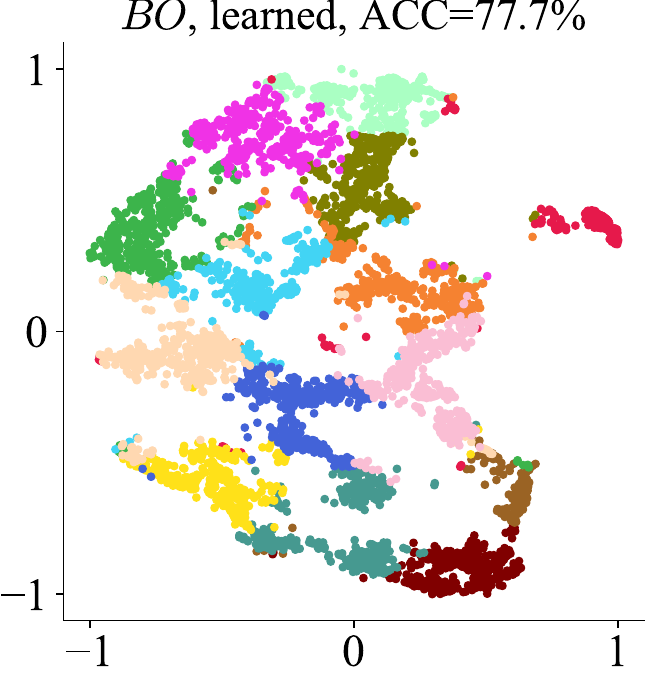}}
  \hfill
  \subfloat[]{\includegraphics[width=0.24\textwidth]{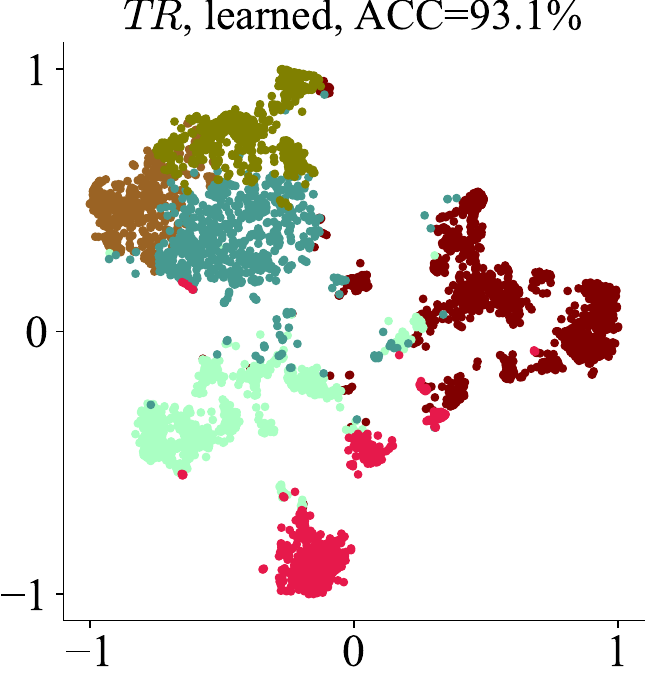}}
  \caption{t-SNE visualizations of superpixel embeddings. First row: raw features, second row: our method learned features. First column: \textit{Indian Pines} (\textit{IP}), second column: \textit{Pavia University} (\textit{PU}), third column: \textit{Botswana} (\textit{BO}), fourth column: \textit{Trento} (\textit{TR}).}
  \label{tsne}
\end{figure}

\newpage

\section{Different Settings for Edge Learning Loss}
In this section, we tested the performance of setting the weight of $\mathcal{L}_E$ ($\beta$) with curriculum. Specifically, we set $\beta$ to start from 0, increase linearly over a certain number of warm-up epochs, and remain constant after reaching the maximum value. Let $\beta_{max}$ denotes the maximum value of $\beta$, and $T_{warm}$ denotes the number of warm-up epochs. Then, $\beta_t$ at the $t$-th epoch is calculated as: 

\begin{equation}
    \beta_t = \frac{\min(t, T_{warm})}{T_{warm}} \cdot \beta_{max}
\end{equation}

\begin{table}[h]
\centering
\caption{Clustering Performance with Different Settings for $\beta$.\label{beta_setting}}
\resizebox{\textwidth}{!}{
\renewcommand\arraystretch{1.14}
\begin{tabular}{c!{\vrule width \lightrulewidth}ccc!{\vrule width \lightrulewidth}ccc!{\vrule width \lightrulewidth}ccc!{\vrule width \lightrulewidth}ccc} 
\toprule
\multirow{2}{*}{\raisebox{-4pt}{Setting}} & \multicolumn{3}{c!{\vrule width \lightrulewidth}}{\textit{Indian Pines}} & \multicolumn{3}{c!{\vrule width \lightrulewidth}}{\textit{Pavia University}} & \multicolumn{3}{c!{\vrule width \lightrulewidth}}{\textit{Botswana}} & \multicolumn{3}{c}{\textit{Trento}}                              \\ 
\cmidrule{2-13}
                        & ACC                 & NMI                 & ARI                          & ACC                 & NMI                 & ARI                              & ACC                & NMI                 & ARI                       & ACC                 & NMI                 & ARI                  \\ 
\midrule
$\beta=0$               & 69.54±1.90          & 70.02±1.30          & 54.79±2.91                   & 68.26±3.36          & \textbf{62.66±3.44} & 54.64±7.43                       & 76.64±1.97         & 82.32±0.92          & 67.93±2.28                & 92.40±1.53          & 89.05±1.42          & 92.86±2.51           \\
$\beta$ with curriculum & 69.86±1.21          & 70.89±0.61          & \textbf{56.12±0.85}          & 69.78±4.03          & 61.93±2.86          & 57.24±8.92                       & \textbf{77.87±1.40} & \textbf{82.91±1.18} & 68.95±2.24                & \textbf{93.14±1.33} & 89.63±1.52          & \textbf{94.11±2.29}  \\
fixed $\beta$           & \textbf{70.01±1.95} & \textbf{71.17±1.31} & 55.99±2.07                   & \textbf{70.00±3.46} & 61.90±3.18          & \textbf{57.26±8.57}              & 77.66±1.28         & 82.90±1.30          & \textbf{69.03±2.38}       & 93.11±0.96          & \textbf{89.74±0.94} & 94.00±1.30           \\
\bottomrule
\end{tabular}}
\end{table}

We performed a grid search over $\beta_{max} \in \{10^{-5},10^{-4},10^{-3},0.01,0.1,1,10\}$ and $T_{warm} \in \{5,10,20,30,40,50,60,70,80,$ $90, 100\}$ to report the best performance. As shown in Table \ref{beta_setting}, the clustering performance achieved by fixed $\beta$ is very close to $\beta$ with curriculum, while the latter introduces one additional hyperparameter. Therefore, we recommend keeping $\beta$ constant during training, which is simple and effective.

\section{Further Sensitivity Analyses}
\subsection{Sensitivity to Superpixel Segmentation Method}

\begin{table}[h]
\centering
\caption{The Influence of Different Superpixel Segmentation Methods.\label{sp_seg_method}}
\resizebox{\textwidth}{!}{
\renewcommand\arraystretch{1.14}
\begin{tabular}{c!{\vrule width \lightrulewidth}ccc!{\vrule width \lightrulewidth}ccc!{\vrule width \lightrulewidth}ccc!{\vrule width \lightrulewidth}ccc} 
\toprule
\multirow{2}{*}{\raisebox{-4pt}{Method}} & \multicolumn{3}{c!{\vrule width \lightrulewidth}}{\textit{Indian Pines}} & \multicolumn{3}{c!{\vrule width \lightrulewidth}}{\textit{Pavia University}} & \multicolumn{3}{c!{\vrule width \lightrulewidth}}{\textit{Botswana}} & \multicolumn{3}{c}{\textit{Trento}}                              \\ 
\cmidrule{2-13}
                        & ACC                 & NMI                 & ARI                          & ACC                 & NMI                 & ARI                              & ACC                 & NMI                 & ARI                      & ACC                 & NMI                 & ARI                  \\ 
\midrule
LSC                     & 65.27±1.69          & 65.33±1.13          & 51.34±1.70                   & 61.64±2.52          & 56.75±3.01          & 43.38±3.08                       & 74.07±2.48          & 80.69±1.04          & 65.91±1.76               & 90.98±3.01          & 86.07±2.59          & 90.60±4.70           \\
SLIC                    & 61.75±2.10          & 64.02±1.07          & 46.43±1.93                   & 62.44±2.05          & 55.95±3.27          & 43.54±5.45                       & 75.02±0.72          & 80.61±1.07          & 64.44±1.62               & 89.53±1.74          & 87.12±1.99          & 90.53±2.45           \\
ERS                     & \textbf{70.01±1.95} & \textbf{71.17±1.31} & \textbf{55.99±2.07}          & \textbf{70.00±3.46} & \textbf{61.90±3.18} & \textbf{57.26±8.57}              & \textbf{77.66±1.28} & \textbf{82.90±1.30} & \textbf{69.03±2.38}      & \textbf{93.11±0.96} & \textbf{89.74±0.94} & \textbf{94.00±1.30}  \\
\bottomrule
\end{tabular}}
\end{table}

We explored the effects of different superpixel segmentation methods (i.e., ERS \cite{ers}, SLIC \cite{slic} and LSC \cite{lsc}) on clustering performance. For each method, we have searched for the optimal number of superpixels ($M$) within the same interval. As shown in Table \ref{sp_seg_method}, ERS achieves the best clustering results on all four datasets. According to ACC, LSC ranks second on \textit{Indian Pines} and \textit{Trento}, while SLIC ranks second on \textit{Pavia University} and \textit{Botswana}. The performance gap between LSC and SLIC is relatively small. Generally, our model is not highly sensitive to different superpixel segmentation methods.

\subsection{Sensitivity to PCA Dimensionality}
\begin{figure}[ht]
  \centering
  \subfloat[]{\includegraphics[width=0.4\textwidth]{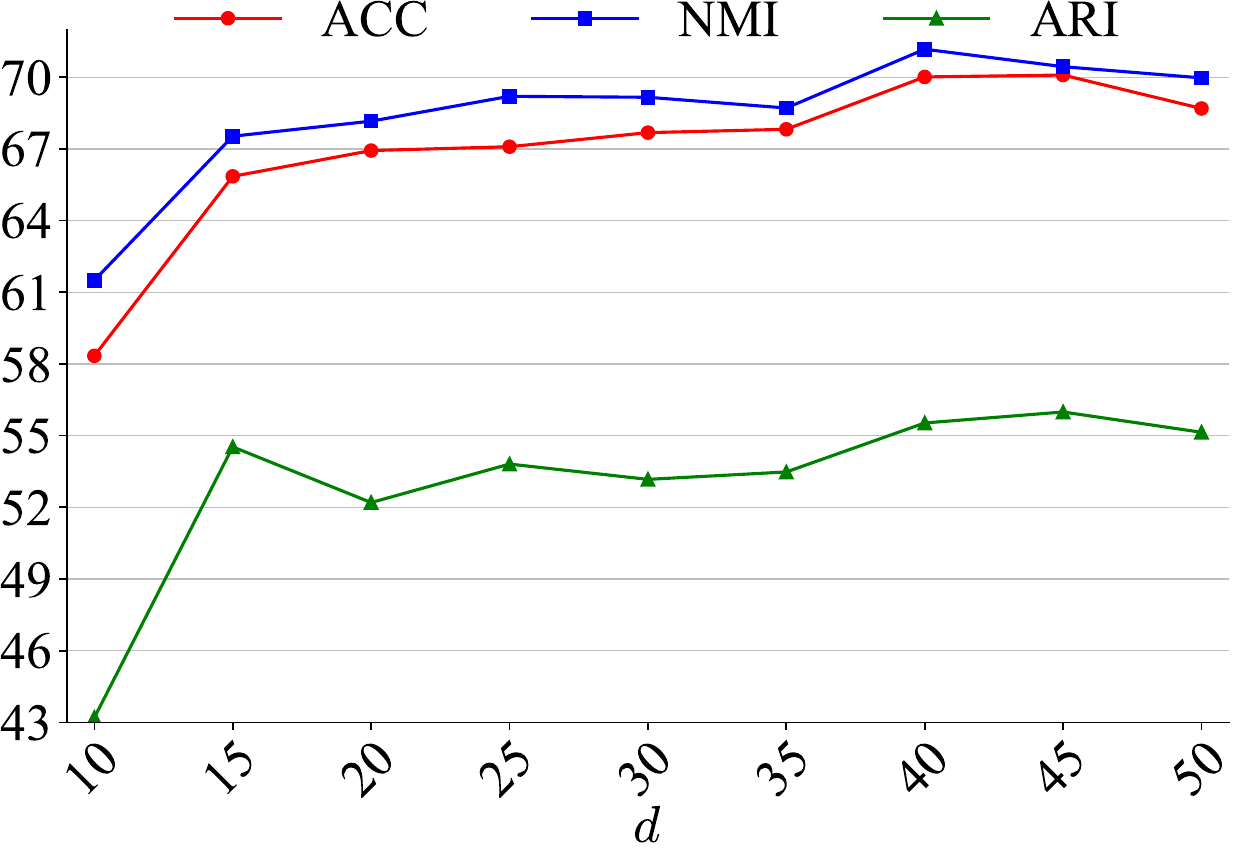}}
  \hspace{0.1\textwidth}
  \subfloat[]{\includegraphics[width=0.4\textwidth]{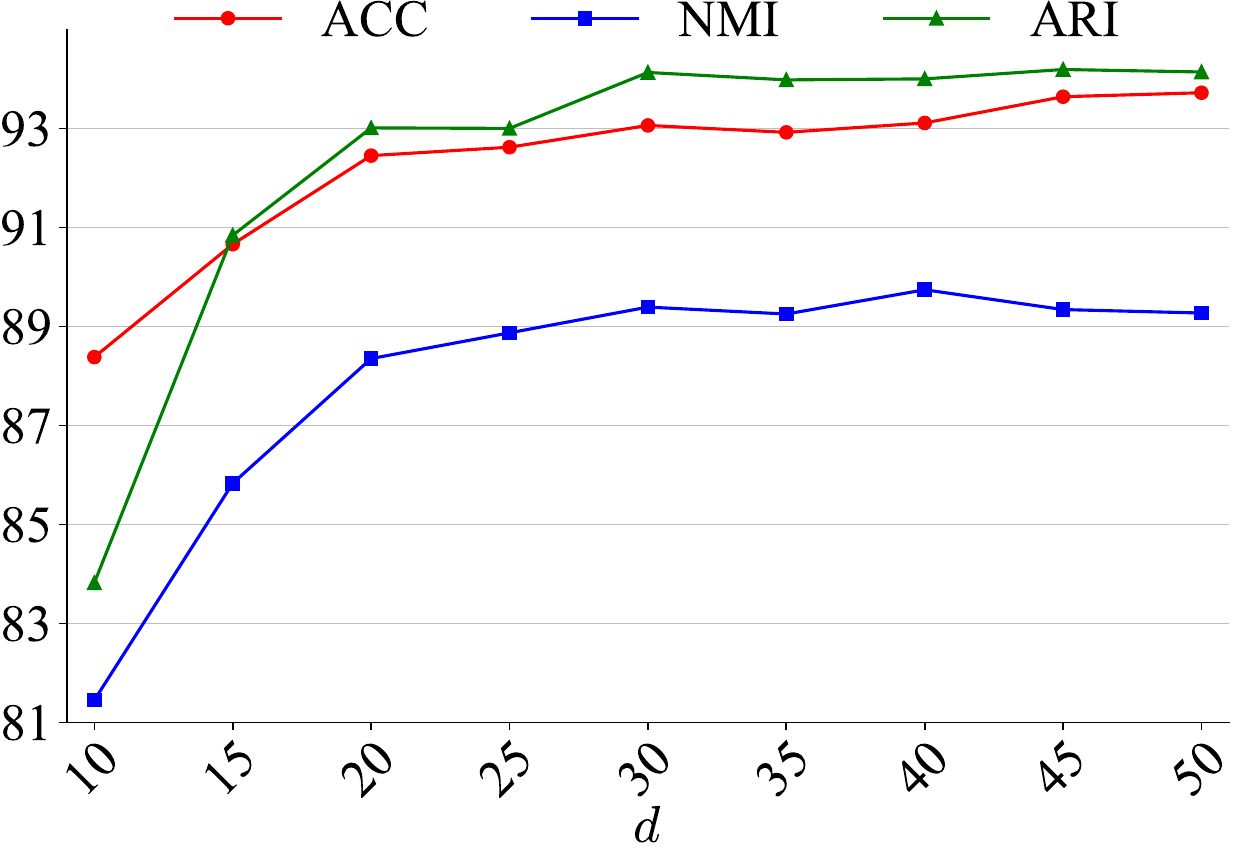}}
  \caption{The influence of different PCA dimensionality ($d$) on: (a) \textit{Indian Pines}, (b) \textit{Trento}.}
  \label{d_influence}
\end{figure}
We conducted a parameter analysis for the PCA dimensionality ($d$), which determines the number of initially retained spectral bands and directly impacts the computational efficiency. We searched for $d$ in [10, 50] with a step of 5 on \textit{Indian Pines} and \textit{Trento}. As shown in Fig. \ref{d_influence}, our method exhibits promising robustness for $d$. When $d$ exceeds 30, the clustering performance is generally satisfactory.

\bibliographystyle{IEEEtran}
\bibliography{supplementary_file_bib}

\vfill
\end{document}
